# Supplementary material for: Joint Planning of Charging Stations and Power Systems for Heavy-Duty Drayage Trucks
Source: arXiv:2403.14866 source file (2024-03-21)
Supplement: Supplementary file 1 [file 8-appendix-with-exact-charger-levels.tex]

\appendices

\section{Linearization of Logical Constraints}
\label{ap:linear}

We introduce new variables $\hat x^{m\uparrow}_{ijt}$ to ensure constraint \eqref{eq:hatx} is satisfied. In contrast to $\hat x^{m}_{ijt}$ that indicates the need for a type $m$ charger, $\hat x^{m\uparrow}_{ijt} = 1$ indicates the need for a type $m$ charger or \textbf{above}. $x^{m}_{ijt}$ and $x^{m\uparrow}_{ijt}$ have logical relationships. For example, suppose we have two choices of candidate chargers, e.g. 350kW and 500kW, their logical relationships are summarized in Table \ref{tab:demo_hatx} subject to different charging power $x_{it}$.

% \begin{table}[]
%     \centering
%     \begin{tabular}{c|c|c|c|c}
%        \toprule
%        Charging Power $x_{it}$ (kW) & $(0, x^{max}\text{]}$ & $(350, x^{max}\text{]}$ & $(0, 350\text{]}$ & $(350, x^{max}\text{]}$\\
%        \midrule
%        Usage Indicator & $\hat x^{1\uparrow}_{ijt}$ & $\hat x^{2\uparrow}_{ijt}$ & $x^{1}_{ijt}$ & $x^{2}_{ijt}$\\
%        \midrule
%        Possible Combinations of Values & 0 & 0 & 0 & 0\\
%                                        & 1 & 0 & 1 & 0\\
%                                        & 1 & 1 & 0 & 1\\
%        \bottomrule
%     \end{tabular}
%     \caption{Illustration of how charger type is determined}
%     \label{tab:demo_hatx}
% \end{table}

\begin{table}[!h]
\caption{Summary of notations for sets, parameters, and decision variables.}
\begin{center}
\begin{threeparttable}
\begin{tabular}{c|c|c|c|c}
       \toprule
       Charging Power $x_{it}$ (kW) & $(0, x^{max}\text{]}^{*}$ & $(350, x^{max}\text{]}$ & $(0, 350\text{]}$ & $(350, x^{max}\text{]}$\\
       \midrule
       Usage Indicator & $\hat x^{1\uparrow}_{ijt}$ & $\hat x^{2\uparrow}_{ijt}$ & $x^{1}_{ijt}$ & $x^{2}_{ijt}$\\
       \midrule
       Possible Combinations of Values & 0 & 0 & 0 & 0\\
                                       & 1 & 0 & 1 & 0\\
                                       & 1 & 1 & 0 & 1\\
       \bottomrule
\end{tabular}
\begin{tablenotes}\footnotesize
\item[*] $x^{max} = 500$kW.
\end{tablenotes}
\end{threeparttable}
\end{center}
\label{tab:demo_hatx}
\end{table}

From Table \ref{tab:demo_hatx}, we can infer that:

\begin{equation}
\hat x^{1}_{ijt} = \hat x^{1\uparrow}_{ijt} - \hat x^{2\uparrow}_{ijt},
\end{equation}
\begin{equation}
\hat x^{2}_{ijt} = \hat x^{2\uparrow}_{ijt},
\end{equation}

The above relationships can be generalized as follows for three or more choices of charger types:

\begin{equation}
\hat x^{m}_{ijt} = \hat x^{m\uparrow}_{ijt} - \hat x^{m+1\uparrow}_{ijt}, \forall m \in M\setminus|M|
\end{equation}
\begin{equation}
\hat x^{|M|}_{ijt} = \hat x^{|M|\uparrow}_{ijt},
\end{equation}

where $\hat x^{m\uparrow}_{ijt}$ is defined as follows:

\begin{equation}
\hat x^{m\uparrow}_{ijt} =
\begin{cases}
    1, & \text{if $\beta_{ijt}(x_{it} - p^{m-1}) > 0$}\\
    0, & \text{otherwise},
\end{cases} 
\label{eq:hat-x-uparrow}
\end{equation}

\eqref{eq:hat-x-uparrow} can be further linearized as follows:

\begin{equation}
\beta_{ijt}(x_{it} - p^{m-1}) \leq G \hat x^{m\uparrow}_{ijt},
\label{eq:hat-x-uparrow-lin1}
\end{equation}

\begin{equation}
\beta_{ijt}(x_{it} - p^{m-1}) \geq -G (1-\hat x^{m\uparrow}_{ijt})+\epsilon,
\label{eq:hat-x-uparrow-lin2}
\end{equation}

\begin{equation}
\hat x^{m\uparrow}_{ijt} = \{0, 1 \}
\label{eq:hat-x-uparrow-values}
\end{equation}

where $G$ is a large positive number and $G \gg \beta_{ijt}(x_{it} - p^{m-1})$. $\epsilon$ is a small positive number and $\epsilon \ll \beta_{ijt}(x_{it} - p^{m-1})$.
